# Supplementary material for: First-order rhombohedral to cubic phase transition in photoexcited GeTe
Source: arXiv:2404.19339 source file (2024-04-30)
Supplement: Supplementary file 1 [file sm.pdf]

# Supplementary Material for: "First-order rhombohedral to cubic phase transition in photoexcited GeTe"

Matteo Furci,[1] Giovanni Marini,[2] and Matteo Calandra[1,2,3]

[1] *Department of Physics, University of Trento, Via Sommarive 14, 38123 Povo, Italy**
[2] *Graphene Labs, Fondazione Istituto Italiano di Tecnologia, Via Morego, I-16163 Genova, Italy*
[3] *Sorbonne Université, CNRS, Institut des Nanosciences de Paris, UMR7588, F-75252 Paris, France*†

## TECHNICAL DETAILS

The density functional theory (DFT) and density functional perturbation theory (DFPT) calculations were performed by using the Quantum ESPRESSO suite [1–3]. We employed optimized norm-conserving Vanderbilt pseudopotentials [4] with Perdew–Burke–Ernzerhof (PBE) generalized gradient approximation [5] for the exchange and correlation functional. In our calculations, the crystal under photoexcitation is characterised by the presence of two independent populations of photoexcited carriers, one composed of electrons in the bottom of the conduction band and the other formed by valence holes in the top of the valence band. The two distributions are represented by two separate Fermi-Dirac distributions. For the detailed construction and calculation of the electronic density, electronic total energy and total energy derivatives we refer the readers to the previous work [3].
Since the existing DFT literature indicates the energy difference between the rhombohedral ($\alpha$) and cubic ($\beta$) phases of GeTe to be $\sim 20 - 40$meV/f.u. [6–8], we used a plane wave energy cutoff and a k-space integration grid such to ensure a convergence tolerance within $\sim 1\,$meV. In the case of non-photoexcited GeTe, a cutoff of $\sim 80\,$Ry for the plane wave expansion and a uniform k-space grid of $16 \times 16 \times 16$ k points satisfied the convergence requirements for both crystalline phases. The photoexcited case instead required more stringent convergence parameters due to the presence of the valence and conduction Fermi surfaces. In particular, denser k-point grids were needed for a proper convergence of the DFPT phonon frequencies. Thus, uniform k-point grids of up to $30 \times 30 \times 30$ were employed for photoexcited GeTe.
In all phonon calculations, the LO/TO splitting was not included. In the case of photoexcited GeTe, the large free carrier concentrations coming form photoexcited electron-hole pairs (see below) provide the screening mechanism necessary to suppress long range Coulomb interactions.

Concerning the stochastic self-consistent harmonic approximation (SSCHA), we considered a $4\times4\times4$ GeTe supercell comprising 128 atoms in total. Since force calculations on an extensive number of supercell configurations were needed, we switched to ultrasoft pseudopotentials with PBE-GGA exchange and correlation functional instead of the previously mentioned choice. In order to speed up the calculation, slightly underconverged parameters for the DFT self-consistency were chosen. More specifically, we employed a $42\,$Ry plane wave energy cutoff and a $2 \times 2 \times 2$ k-point grid in the supercell DFT calculations. This choice is expected to introduce a systematic error of $\sim 2\,$meV is the determination of GeTe free energy per unit cell. Nonetheless, this is not expected to qualitatively change the results reported as only free energy differences were taken into consideration.

## K-PATH SELECTION IN THE FIRST BRILLOUIN ZONE

In this section, we show explicitly the first Brillouin zones of both $\alpha$- and $\beta$-GeTe (Figure 1). Together with them, we also highlight the k-space path followed when plotting the dispersion relation of the harmonic phonons and of the eigenvalues of the anharmonic hessian matrix. This helps clarifying the labelling of the high symmetry points for the GeTe phases which is fairly different despite the two brillouin zones being almost identical. Here, the high symmetry lines and the labelling of the high symmetry points in k-space follows that of Ref. [9].

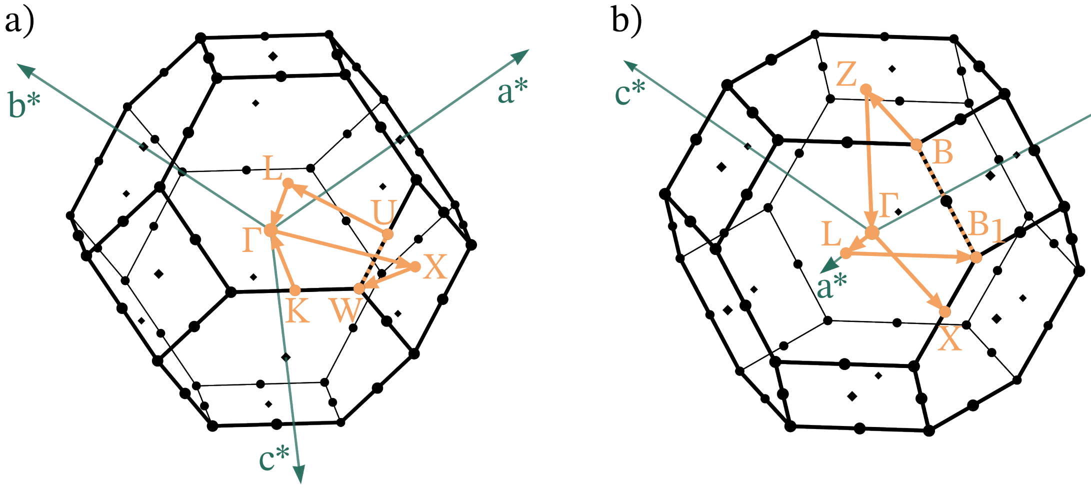


FIG. 1. First Brillouin zones of $\beta$-GeTe (a) and of $\alpha$-GeTe (b). The path followed in plotting the dispersion relations are highlighted in orange. The images were created through the XCrysDen software [10].

## EFFECT OF INTRINSIC HOLE CONCENTRATION ON THE DYNAMICAL INSTABILITY AT $\Gamma$

As found in both theoretical and experimental investigations [11, 12], at finite $T$ intrinsic vacancies in cubic GeTe lead to the presence of quite large free carrier (holes) concentrations, typically from $\sim 1\times10^{19}\text{cm}^{-3}$ up to $\sim 1\times10^{21}\text{cm}^{-3}$ (a value of $7.77(8)\times10^{20}\,\text{cm}^{-3}$ is reported in the experimental work of Ref. [12]). In Ref. [12], the formation of vacancies with increasing temperature was actually also related to a clear although weak first order character of the thermal phase transition. Thus the role of intrinsic hole concentration is undoubtedly relevant for the problem at hand. Despite all of this, the intrinsic hole concentrations are small when compared with the photoexcited electron-hole concentrations in materials undergoing modern ultrafast photoexcitation experiments, as shown in the section "Photoexcited Carrier Concentration" below. A back-of-the-envelope calculation indicates that for GeTe intrinsic hole concentration of 1-100$\times10^{19}$ cm$^{-3}$ amount to $\sim$ 0.0006-0.06 holes/f.u., which are generally lower than the photoexcited electron concentrations considered in this work. Anyway, the effect of these characteristic hole concentrations can be readily checked by performing harmonic phonon calculations in the presence of a uniform hole doping matching the hole concentrations estimated above and by using a compensating uniform charge density background. For the sake of simplicity, we only report here the dependence of the optical zone center mode of the cubic phase as a function of hole concentration. The results are depicted in Fig.2. As it can be noted, even at the largest hole concentration,

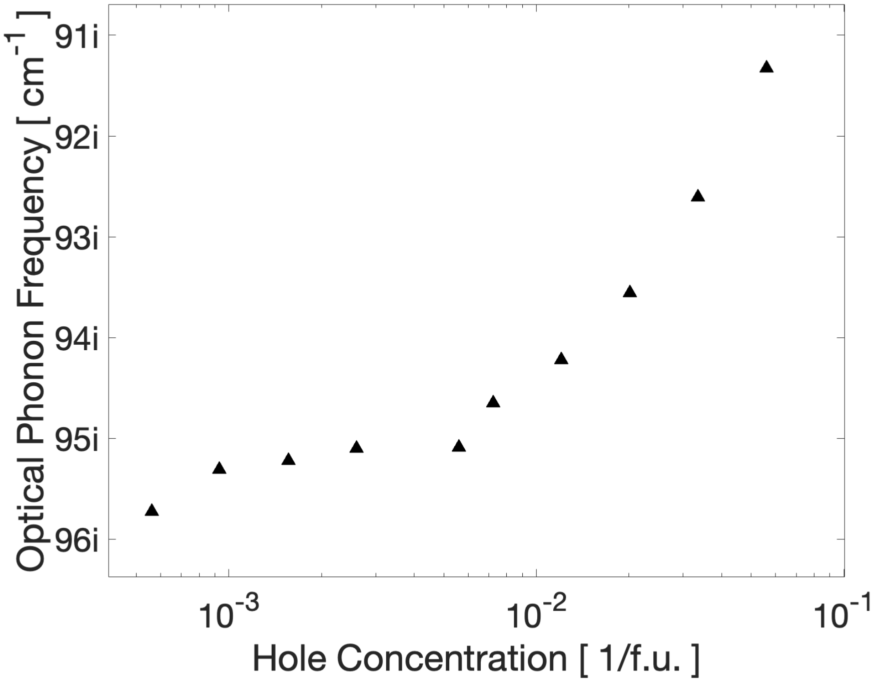


FIG. 2. Harmonic optical phonon frequency for $\beta$-GeTe as a function of hole doping concentration.

the dynamical instability at $\Gamma$ is only slightly reduced ($\approx$ 5%) with respect to the perfectly stoichiometric compound. Thus, the inclusion of the intrinsic hole concentration does not affect the conclusion of the present work.

## PROJECTED BAND CHARACTER IN CUBIC GETE

The projection over the Ge and Te atomic character of the electronic structure of cubic GeTe provide the same information as showed in the main text for rhombohedral GeTe. In Figure 3, the projection over the Ge (top) and Te (bottom) atomic states is reported.

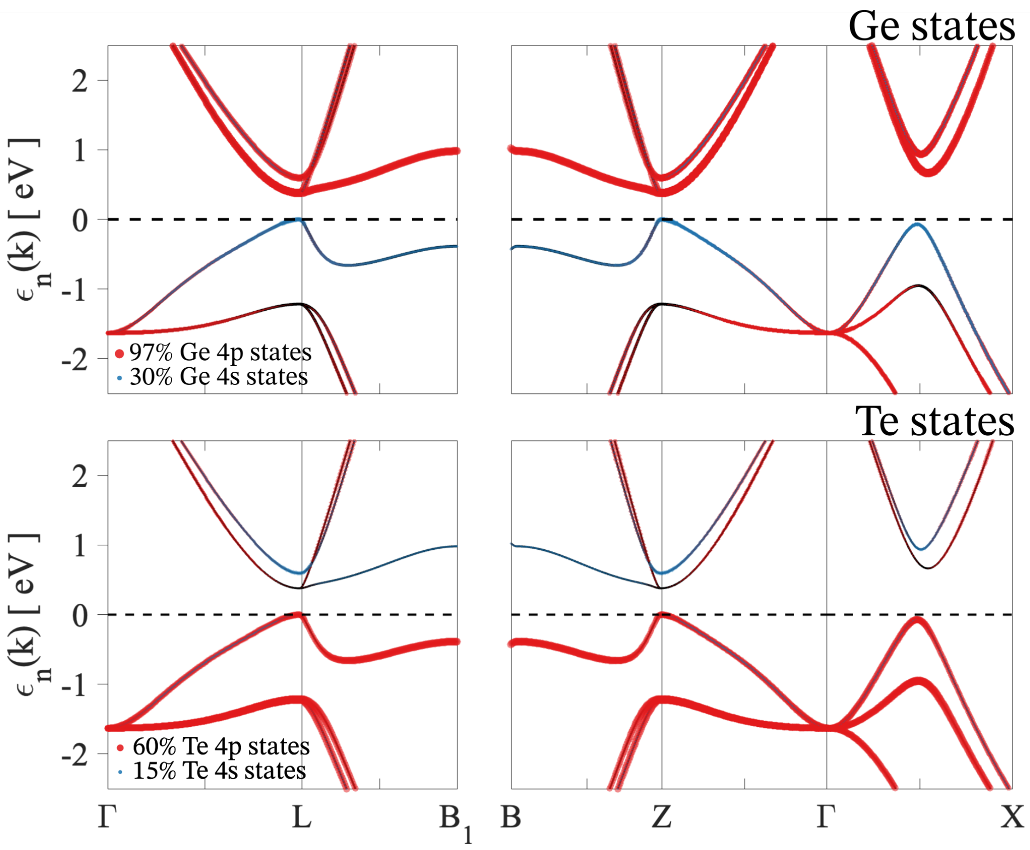


FIG. 3. Projections over the Ge (top) and Te (bottom) atomic states plotted over the electronic band structure of ground state $\beta$-GeTe. The path in k-space chosen to plot the electronic band structure is the same employed for $\alpha$-GeTe. The rhombohedral Brillouin zone labelling was employed, according to the cubic brillouin zone labelling one has the following associations: $B_1$, $B \rightarrow W$, $Z \rightarrow L$ and $X \rightarrow K$.

Once again, even for cubic GeTe, the bottom of the conduction band is predominantly of Ge character, with up to 97% Ge character at the bottom of the conduction band at $L$. The top of the valence band has a slightly more dominant Te character instead.

## DFT BANDGAP UNDER PHOTOEXCITATION

We provide in Figure 4 the behaviour of the DFT fundamental bandgaps of both rhombohedral and cubic GeTe as a function of increasing photoexcited carrier concentration. As shown in the main text, the single particle bandgap of the $\alpha$ phase is strongly affected by photoexcitation and closes already at $n_e = 0.15\text{e}^-/\text{f.u.}$. Figure 4 clearly shows instead how the cubic structure bandgap is not sensitive to the presence of photoexcited carrier in the conduction bands, remaining approximately constant at all concentration considered. The bandgap of the cubic phase is protected by symmetry as the angle between the primitive cell lattice vectors is fixed by the cubic structure.

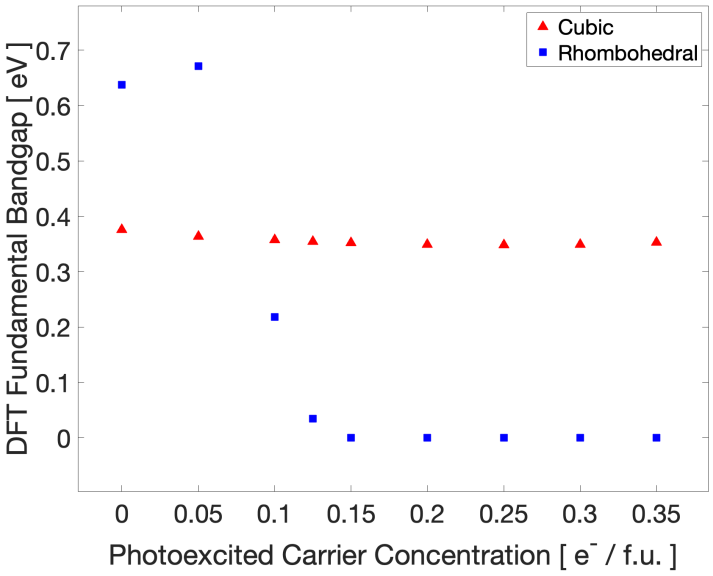


FIG. 4. Simulated density functional theory fundamental gap in both $\alpha$- and $\beta$-GeTe as a function of increasing photoexcition.

## PHOTOEXCITED CARRIER CONCENTRATION

We provide here an estimate of the number of photoexcited electron-hole pairs populating the valence and conduction bands of GeTe after the initial pumping in the experiment of Ref. [13]. We roughly follow the same line of reasoning proposed by Ref. [14] which dealt with the same problem in the case of Ge-Sb-Te alloys.
In Ref. [13], the authors deal with a polycrystalline thin film of GeTe with thickness $z_0 = 40\,\text{nm}$. Taking into account the progressive attenuation of the electromagnetic radiation inside the material, we can estimate the average laser fluence $\bar{F}$ which the thin film is subject to through the following

$$\bar{F} = (1 - R(\omega_\text{L}))\,\frac{1}{z_0}\int_0^{z_0} F e^{-\alpha(\omega_\text{L})z}\,dz, \tag{1}$$

where $F$ is the original laser fluence at the thin film surface, $\omega_\text{L}$ its frequency and $R(\omega_\text{L})$ and $\alpha(\omega_\text{L})$ are the reflection and the optical absorption coefficients of GeTe respectively.
Assuming the radiation intensity to be sufficiently small, the average number of photoexcited electron-hole pairs per unit volume $\bar{N}_{\text{e}-\text{h}}$ can be readily estimated as

$$\bar{N}_{\text{e}-\text{h}} = \frac{\alpha(\omega_\text{L})\,\bar{F}}{\hbar\omega_\text{L}}. \tag{2}$$

The experimental values of the quantities appearing in Equations (1) and (2) are: $F = 20\,\text{mJ}\,\text{cm}^{-2}$ [13], $\omega_\text{L} = 800\,\text{nm}$ ($\hbar\omega_\text{L} \simeq 1.55\,\text{eV}$) [13], $R(\omega_\text{L}) \simeq 0.6$ [15] and $\alpha(\omega_\text{L}) = 4 \times 10^5\,\text{cm}^{-1}$. Plugging everything into the equations above gives

$$\bar{N}_{\text{e}-\text{h}} = 6.6 \times 10^{21}\,\text{cm}^{-3} \simeq 0.36\,\text{e}^-/\text{f.u.}. \tag{3}$$

where in the last equation the photoexcited electron-hole pair density was multiplied by the volume of the GeTe primitive cell $V \simeq 55\,\text{Å}^3 = 55 \times 10^{-24}\,\text{cm}^3$.
The estimated concentration of photoexcited electrons is of the same order of the values used for the simulations of photoexcited GeTe presented in the main, albeit somewhat larger. It should be noted however that the present estimate does not take into account saturating absorption effects beyond our linear approximation and is thus only an upper bound for the concentration of the photoexcited electrons in the material
We conclude that the choice of $n_\text{e} = 0.1\,\text{e}^-/\text{f.u.}$ as concentration of photoexcited electrons in the material represents a reasonable estimate of the actual average concentration in the experimental sample.

## PHONON SPECTRAL FUNCTION

In this section, we show the full dynamic spectral function of the vibrational degrees of freedom of photoexcited cubic GeTe ($n_{\mathrm{e}} = 0.1\,\mathrm{e}^{-}/\mathrm{f.u.}$). In particular, the SSCHA code provides the spectral function for each phonon mode $\mu$ as

$$\sigma_{\mu}\left(\mathbf{q},\Omega\right) = \frac{1}{2}\left[\frac{1}{\pi}\frac{-\mathrm{Im}\mathcal{Z}_{\mu}\left(\mathbf{q},\Omega\right)}{\left[\Omega-\mathrm{Re}\mathcal{Z}_{\mu}\left(\mathbf{q},\Omega\right)\right]^{2}+\left[\mathrm{Im}\mathcal{Z}_{\mu}\left(\mathbf{q},\Omega\right)\right]^{2}}+\frac{1}{\pi}\frac{\mathrm{Im}\mathcal{Z}_{\mu}\left(\mathbf{q},\Omega\right)}{\left[\Omega-\mathrm{Re}\mathcal{Z}_{\mu}\left(\mathbf{q},\Omega\right)\right]^{2}+\left[\mathrm{Im}\mathcal{Z}_{\mu}\left(\mathbf{q},\Omega\right)\right]^{2}}\right], \tag{4}$$

where $\mathbf{q}$ is a vector in the first Brillouin zone and $\Omega$ is the energy variable; $\mathcal{Z}_{\mu}\left(\mathbf{q},\Omega\right)$ is defined as

$$\mathcal{Z}_{\mu}\left(\mathbf{q},\Omega\right) = \sqrt{\omega_{\mu}^{2}\left(\mathbf{q}\right)+\Pi_{\mu\mu}\left(\mathbf{q},\Omega\right)} \tag{5}$$

with $\omega_{\mu}\left(\mathbf{q}\right)$ being the eigenvalue of the anharmonic force constant matrix and $\Pi_{\mu\mu}\left(\mathbf{q},\Omega\right)$ being the diagonal element of the self energy of the SSCHA phonons [14].
In Figure 5, the full spectral function summed over all phonon modes is plotted as a colourplot on the dispersion relation of the eigenvalues of the anharmonic hessian matrix of photoexcited cubic GeTe ($n_{\mathrm{e}} = 0.1\,\mathrm{e}^{-}/\mathrm{f.u.}$). In Figure 6 the spectral function at zone centre is plotted.

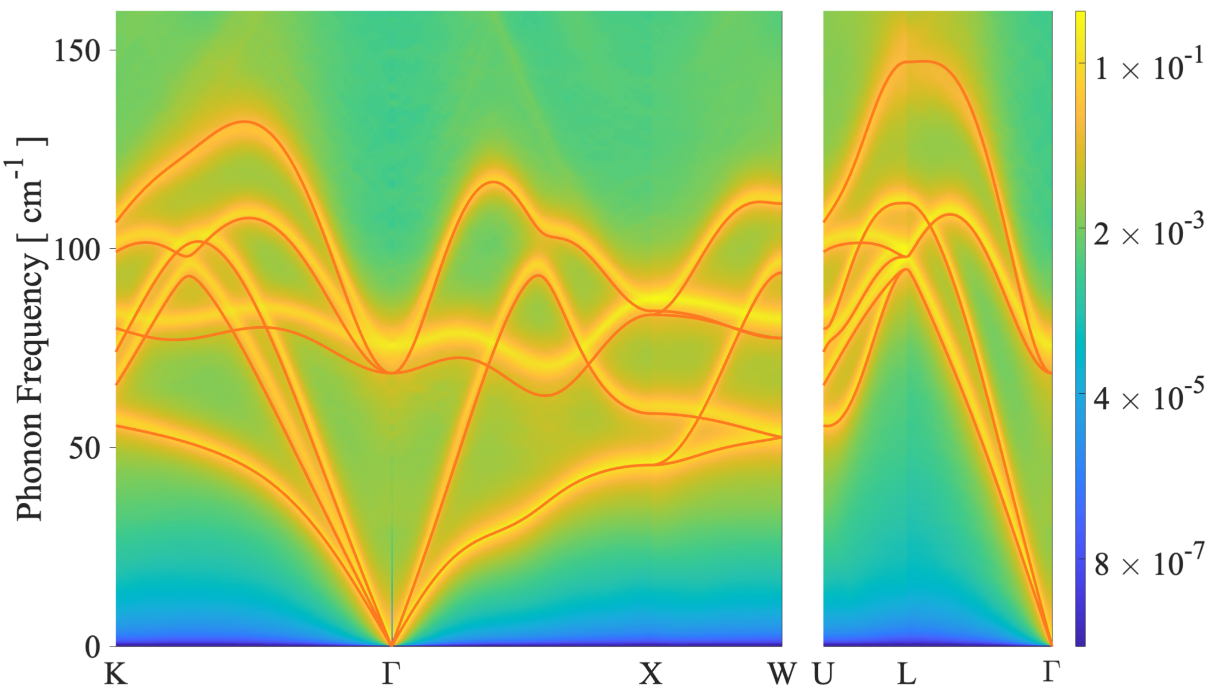


FIG. 5. Full spectral function for photoexcited cubic GeTe at $n_{\mathrm{e}} = 0.1\,\mathrm{e}^{-}/\mathrm{f.u.}$; solid lines represent the dispersion relation of the eigenvalues of the anharmonic hessian matrix.

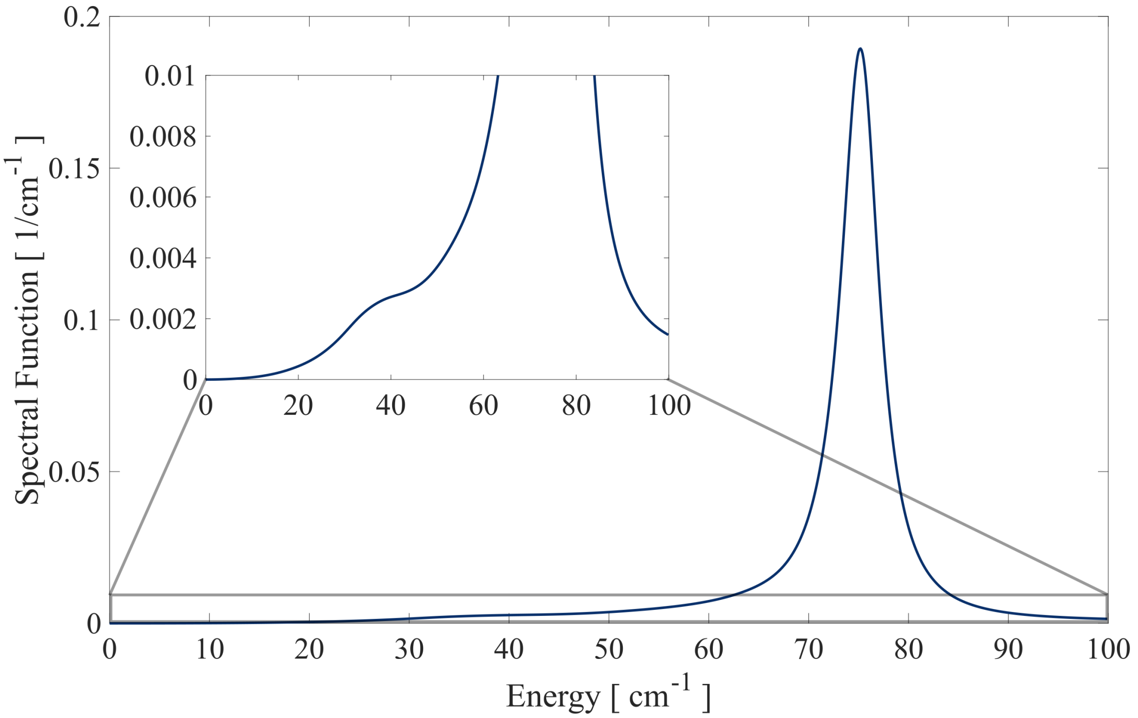


FIG. 6. Spectral function for photoexcited cubic GeTe at $n_\mathrm{e} = 0.1\,\mathrm{e}^{-}/\mathrm{f.u.}$ for $\mathbf{q} = 0$.

The peaks in the spectral weight do not coincides with the eigenvalues of the positional free energy Hessian. Moreover additional structure in the energy spectrum at $\Gamma$ can be seen forming at roughly $40\,\mathrm{cm}^{-1}$.

## DIFFRACTION PEAKS

### Volume correction for the ground state spectra

Residual structures contributing to the asymmetry of the diffraction peaks of photoexcited GeTe in Ref. [13] suggest a possible coexistence of the rhombohedral and cubic phase. In this section, we detail the comparison between the diffraction peaks in the phase coexistence scenario and the experimental ones reported by Ref. [13]. The set of peaks in the reference involve the peaks within the ranges ($2\sin\theta/\lambda$) of: [2.6, 3.2] $\mathrm{cm}^{-1}$, [3.2, 3.6] $\mathrm{cm}^{-1}$ and [4.4, 5.0] $\mathrm{cm}^{-1}$. As in the main text, we restrict ourselves to the first and last set of peaks as the remaining one ([012] peak in hexagonal representation) is left almost invariant under a rhombohedral to cubic transformation of the lattice.

We first focus on the experimental diffraction pattern corresponding to non-photoexcited rhombohedral GeTe. The latter is compared with the theoretical peaks of the DFT structure given by the VESTA software [16]. In order to ease the comparison, we performed a linear fit of the tails of the experimental signals and removed the background noise which appears to steadily increase at lower diffraction angles. Subsequently, we also performed a gaussian fit so to extract the experimental half width at half maximum (HWHM). The broadening given by the extracted HWHM were then superimposed on the theoretical peaks given by VESTA. In Figure 7, we show the result of this analysis. All the curves were normalized to unity in their respective window of $2\sin\theta/\lambda$.

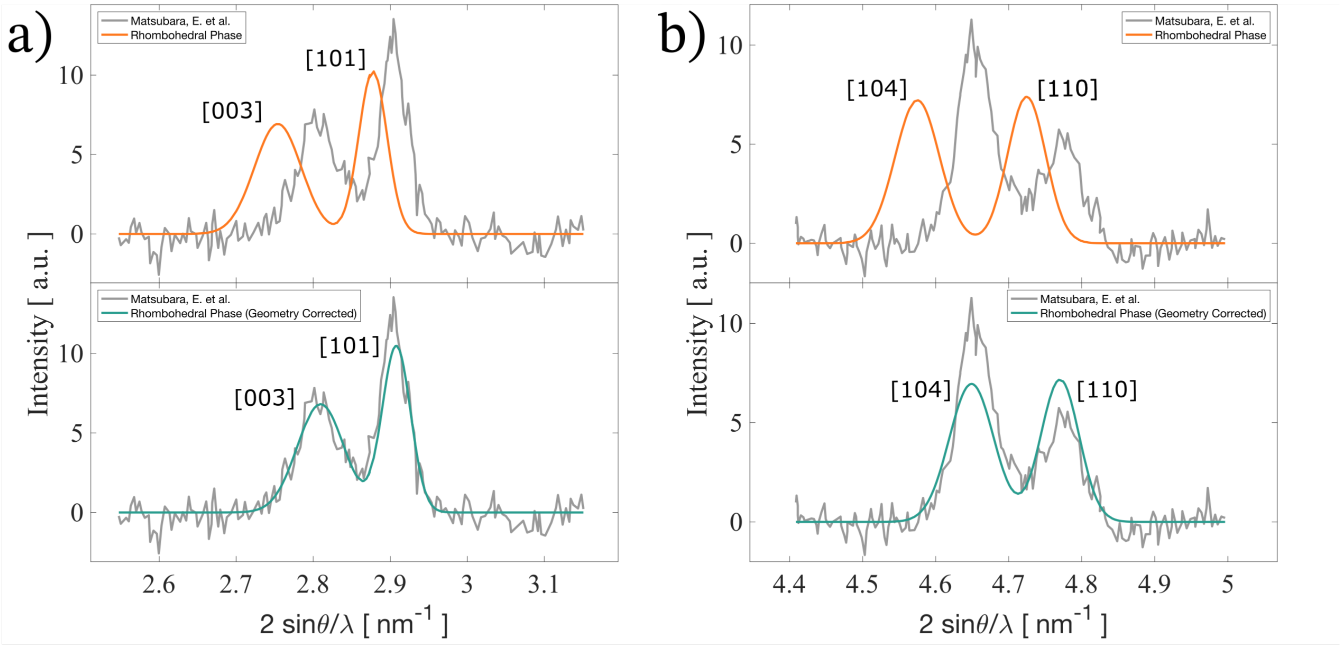


FIG. 7. Comparison between the experimental diffraction pattern of ground state $\alpha$-GeTe [13] and the theoretical diffraction patterns corresponding to the DFT structure of $\alpha$-GeTe as obtained from plain geometry optimization (top) and as obtained correcting the geometry parameters (bottom). Figure (a) refers to the set of peaks in the range [2.6, 3.2] $\mathrm{cm}^{-1}$ of $2\sin\theta/\lambda$; Figure (b) refers instead to the range [4.4, 5.0] $\mathrm{cm}^{-1}$ of $2\sin\theta/\lambda$. The position of the diffraction peaks for the simulated structures is obtained through the VESTA software [16].

The VESTA diffraction pattern is fairly close to the experimental one, however discrepancies in the position and spacing of the peaks are still evident due to the extreme sensitivity to the lattice geometry of Xray diffraction measurements (top row of Figure 7). Nonetheless, a reduction of 3.8% of the unit cell volume and an increase of $\sim 0.7\%$ of the rhombohedral angle are sufficient to restore an excellent agreement with the experiment, as shown in the bottom row of Figure 7. These errors in the lattice geometry are within the usual accuracy of DFT geometry optimization.

## Volume relaxation effect on the photoexcited spectra

One may wonder whether the inclusion of photoinduced volume relaxation effects improves or worsens the agreement shown in Fig.6 of the main text between our simulations and the photoexcited diffraction signal. Indeed, since time resolved measurements in Ref. [13] were taken after few ps, photoinduced volume changes may already have propagated in the sample. To verify this possibility, we repeated the simulations presented in Fig. 6 of the main text including the volume relaxation effects due to the presence of a photoexcited carrier concentration of $n_{\mathrm{e}} = 0.1\,\mathrm{e}^{-}/\mathrm{f.u.}$. As in Fig.6 of the the main text, we compare the experimental curves with the theoretical diffraction pattern originating from the rhombohedral phase, the cubic phase and a mixture of the two. The latter is taken here as a weighted sum of the diffraction intensities of the two phases in the mixture

$$I_{\mathrm{mixture}} = \left[(1-\alpha) I_{\alpha-\mathrm{GeTe}} + \alpha I_{\beta-\mathrm{GeTe}}\right]/N \tag{6}$$

with $\alpha \in [0, 1]$ and $N$ being a normalization factor so that we can work with diffraction pattern normalized to unity. In Figure 8, the comparison is shown for the same cubic concentration $\alpha$ used in Figure 6 of the main text.

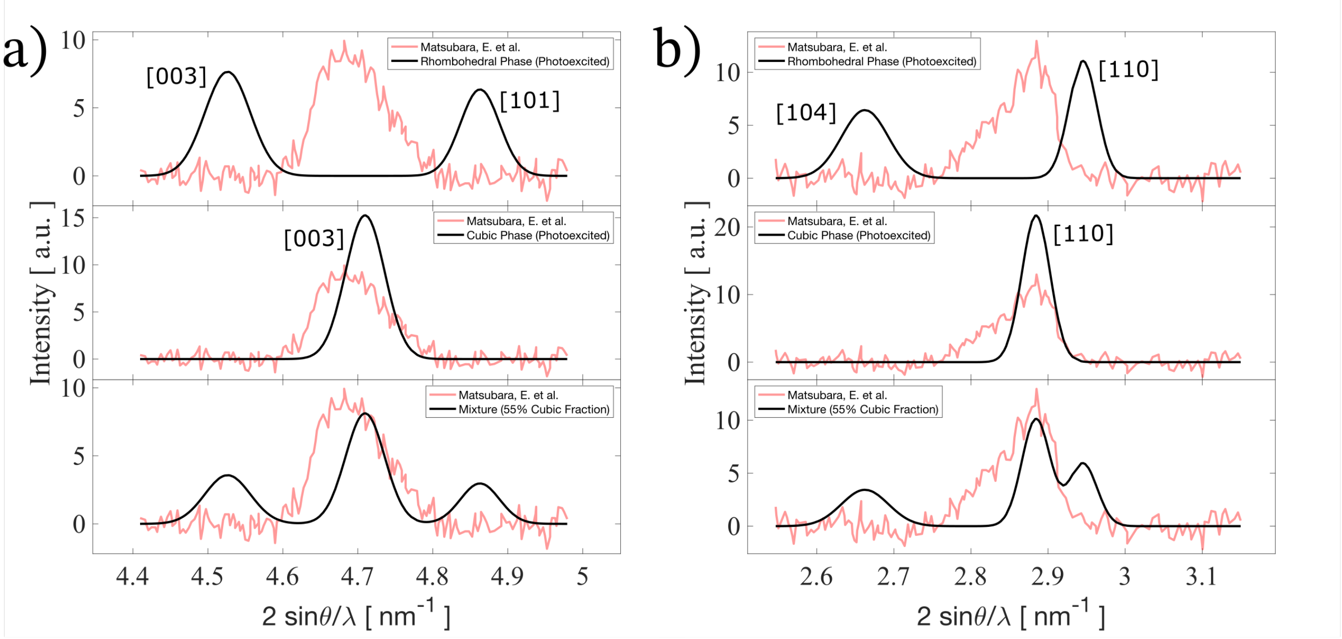


FIG. 8. Comparison between the experimental diffraction pattern of photoexcited GeTe at 6 ps [13] and the theoretical diffraction patterns corresponding to the photoexcited structures simulated through DFT. From top to bottom, the diffraction pattern of photoexcited $\alpha$-Gete ($n_\mathrm{e} = 0.1\,\mathrm{e}^-/\mathrm{f.u.}$), of photoexcited $\beta$-GeTe ($n_\mathrm{e} = 0.1\,\mathrm{e}^-/\mathrm{f.u.}$) and of a coexistence of the two are reported respectively. Figure (a) refers to the set of peaks in the range [2.6, 3.2] $\mathrm{cm}^{-1}$ of $2\sin\theta/\lambda$; Figure (b) refers instead to the range [4.4, 5.0] $\mathrm{cm}^{-1}$ of $2\sin\theta/\lambda$. The position of the diffraction peaks for the simulated structures is obtained through the VESTA software [16].

The peak broadening for the rhombohedral diffraction patterns are the same as those obtained from gaussian fitting of the ground state peaks. The broadening of the single cubic peak in each of the two window of $2\sin\theta/\lambda$ are instead chosen to be the smallest between the HWHMs of the two rhombohedral peaks present in the same window.
From Figure 8, it is clear that the inclusion of volume relaxation effects worsens the agreement with the experimental data. Most specifically, the geometry of photoexcited rhombohedral GeTe gives a peak spacing too large to combine with the single cubic peak and give rise to the observed asymmetry of the diffraction peaks. Indeed, although the rhombohedral volume of photoexcited $\alpha$-GeTe is only 1% smaller than the theoretical ground state volume, the rhombohedral angle of the photoexcited rhombohedral structure decreases by 5% thus giving rise to an enhanced splitting of the rhombohedral diffraction peaks.

As presented in the main text, a better agreement is found when mixing the diffraction pattern of photoexcited cubic GeTe with the diffraction pattern of ground state rhombohedral GeTe (Figure 6 of the main text), indicating that the fraction of rhombohedral GeTe in the sample is still characterized by its ground state volume at 6 ps.

We conclude this section by mentioning how the cubic fraction in sample best explaining the experimental data is found. We consider the whole range of possible cubic fractions $\alpha$ in the system and construct the corresponding mixed diffraction pattern as according to (6). Presently, we mix the theoretical diffraction pattern of ground state rhombohderal GeTe and that of photoexcited cubic GeTe ($n_\mathrm{e} = 0.1\,\mathrm{e}^-/\mathrm{f.u.}$). In order to find the optimal $\alpha$, we minimize the integrated square deviation of the theoretical diffraction pattern form the experimental one

$$\Delta = \int \left| I_\mathrm{th}(x) - I_\mathrm{exp}(x) \right|^2 \, dx \tag{7}$$

where $I_\mathrm{th}(x)$ and $I_\mathrm{exp}(x)$ are the theoretical and experimental diffraction intensity as a function of $x = 2\sin\theta/\lambda$. In Figure 9 we report the integrated square error $\Delta$ as a function of the cubic fraction in the sample $\alpha$ for both set of of peaks considered here. Taking the average of the two found minima we obtain a cubic fraction in the sample of 55%.

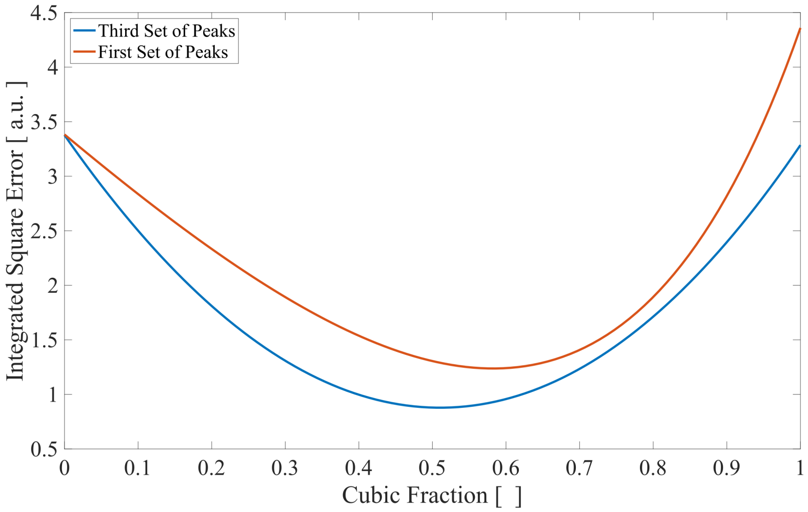


FIG. 9. Integrated square error of the theoretical photoexcited diffraction pattern compared with the experimental one. The first set of peaks indicates the set of peaks in the range [2.6, 3.2] $cm^{-1}$ of $2\sin\theta/\lambda$, whereas the third set of peaks indicates those in the range [4.4, 5.0] $cm^{-1}$ of $2\sin\theta/\lambda$.

* matteo.furci@unitn.it
† m.calandrabuonaura@unitn.it

[1] P. Giannozzi, S. Baroni, N. Bonini, M. Calandra, R. Car, C. Cavazzoni, D. Ceresoli, G. L. Chiarotti, M. Cococcioni, I. Dabo, A. D. Corso, S. de Gironcoli, S. Fabris, G. Fratesi, R. Gebauer, U. Gerstmann, C. Gougoussis, A. Kokalj, M. Lazzeri, L. Martin-Samos, N. Marzari, F. Mauri, R. Mazzarello, S. Paolini, A. Pasquarello, L. Paulatto, C. Sbraccia, S. Scandolo, G. Sclauzero, A. P. Seitsonen, A. Smogunov, P. Umari, and R. M. Wentzcovitch, Journal of Physics: Condensed Matter **21**, 395502 (2009).
[2] P. Giannozzi, O. Baseggio, P. Bonfà, D. Brunato, R. Car, I. Carnimeo, C. Cavazzoni, S. de Gironcoli, P. Delugas, F. Ferrari Ruffino, A. Ferretti, N. Marzari, I. Timrov, A. Urru, and S. Baroni, The Journal of Chemical Physics **152**, 154105 (2020).
[3] G. Marini and M. Calandra, Phys. Rev. B **104**, 144103 (2021).
[4] D. R. Hamann, Phys. Rev. B **88**, 085117 (2013).
[5] J. P. Perdew, K. Burke, and M. Ernzerhof, Phys. Rev. Lett. **78**, 1396 (1997).
[6] T. Chatterji, C. M. N. Kumar, and U. D. Wdowik, Phys. Rev. B **91**, 054110 (2015).
[7] D. Lencer, M. Salinga, B. Grabowski, T. Hickel, J. Neugebauer, and M. Wuttig, Nature Materials **7**, 972 (2008).
[8] U. D. Wdowik, K. Parlinski, S. Rols, and T. Chatterji, Phys. Rev. B **89**, 224306 (2014).
[9] W. Setyawan and S. Curtarolo, Computational Materials Science **49**, 299 (2010).
[10] A. Kokalj, Journal of Molecular Graphics and Modelling **17**, 176 (1999).
[11] A. H. Edwards, A. C. Pineda, P. A. Schultz, M. G. Martin, A. P. Thompson, and H. P. Hjalmarson, Journal of Physics: Condensed Matter **17**, L329 (2005).
[12] M. Sist, H. Kasai, E. M. J. Hedegaard, and B. B. Iversen, Phys. Rev. B **97**, 094116 (2018).
[13] E. Matsubara, S. Okada, T. Ichitsubo, T. Kawaguchi, A. Hirata, P. F. Guan, K. Tokuda, K. Tanimura, T. Matsunaga, M. W. Chen, and N. Yamada, Phys. Rev. Lett. **117**, 135501 (2016).
[14] L. Monacelli, R. Bianco, M. Cherubini, M. Calandra, I. Errea, and F. Mauri, Journal of Physics: Condensed Matter **33**, 363001 (2021).
[15] J. E. Lewis, physica status solidi (b) **59**, 367 (1973).
[16] K. Momma and F. Izumi, Journal of Applied Crystallography **44**, 1272 (2011).
